# Supplementary material for: Bayesian Inference for Generalized Linear Model with Linear Inequality Constraints
Source: arXiv:2108.10472 source file (2021-08-24)
Supplement: Supplementary file 1 [file supplba-template.tex]

%\RequirePackage{etoolbox}
%\csdef{input@path}{%
% {sty/}% cls, sty files
% {img/}% eps files
%}%
%\csgdef{bibdir}{bib/}% bst, bib files

\documentclass[12 pt]{article}
%
%\pubyear{0000}
%\volume{00}
%\issue{0}
%\doi{0000}
%\firstpage{1}
%\lastpage{1}


%
\usepackage{amsthm}
%\usepackage{amsmath}
\usepackage{amsmath, amssymb}
\usepackage{natbib}
\usepackage[colorlinks,citecolor=blue,urlcolor=blue,filecolor=blue,backref=page]{hyperref}
\usepackage{graphicx}
\usepackage{bbold}
\usepackage{mathbbol}
\usepackage{float}
\usepackage{algorithm}
\usepackage{algorithmic}
\usepackage{enumitem}
\usepackage{multirow}
\usepackage{bm} % Math packages
\usepackage{float}
\def\*#1{\mathbf{#1}}
%\def\^#1{\amsmathbb{#1}}
\def\^#1{\mathbf{#1}}
\def\##1{\mathbb{#1}}
\DeclareSymbolFontAlphabet{\amsmathbb}{AMSb}%
\renewcommand{\thefigure}{S\arabic{figure}}
\renewcommand{\thetable}{S\arabic{table}}


\begin{document}

%% *** Frontmatter *** 


\title{Supplementary Material for ``Bayesian Inference for Generalized Linear Model with Linear Inequality Constraints"}
\author{Rahul Ghosal and
Sujit Ghosh\\[4pt]
}
\date{}
\maketitle
%\title{\thanksref{T1}}
%\thankstext{T1}{<thanks text>}


%% ** Mainmatter **

%\section{}\label{}

% \begin{figure} 
% \includegraphics{<eps-file>}% place <eps-file> in ./img  subfolder
% \caption{}
% \label{}
% \end{figure}


% \begin{table} 
% *****************
% \begin{tabular}{lll}
% \end{tabular}
% *****************
% \caption{}
% \label{}
% \end{figure}


%% ** The bibliograhy **
\section{Appendix 1: Linear Inequality Constrained Generalized Linear Model
with Binding Constraints}
\label{sec:introsup}
We illustrate the estimation method in linear inequality constrained GLM (Linear model) under the presence of binding or equality constraints. This can be done similarly as in \cite{davis1978bayesian}. We are interested in the constrained parameter space $\Omega= \{\bm\beta: \^R\bm\beta \geq \*b\}$. The constraint matrix $\^R$ is a $m$ by $p$ matrix and can be partitioned as $\^R=[\^R^0 \hspace{3 mm}0]$, where $\^R^0$ is a $m$ by $q$ matrix of active constraints on the parameters. Correspondingly, $\bm\beta$ is partitioned as $\bm\beta=(\bm\beta_1^T \hspace{2 mm}\bm\beta_2^T)^T$. Now w.l.g assume first $m-k$ constraints are binding among the $m$ constraints $\^R^0\bm\beta_1\geq \*b$. Then the set of $\bm\beta$ satisfying the above constraints lie on a $\alpha= p- (m-k)$ dimensional hyperplane. Therefore to asses prior distribution, we eliminate $m-k$ of the restricted variables and obtain an $\alpha$ dimensional vector $\bm\gamma$ which is not degenerate and satisfies equivalent inequality constraint $\^D\bm\gamma \geq \*w$. Then the proposed method in Section 2.2 in the paper can be applied for estimation under such linear inequality constraints.
We present a brief proof below. 

Let $1\leq m-k \leq q$, this is the case we are interested in, the constraints on $\bm\beta_1$ is
\begin{align}
    \^R^{s}\bm\beta_1&=\* b_s\textit{ where $\* b_s^T=(b_1,\ldots,b_{m-k})$, $\^R^s_{(m-k)\times q}$ are the binding constraints, }  \label{eq:1}\\
    \^G^{s}\bm\beta_1&>\* g_s \textit{ where $\* g_s^T=(b_{m-k+1},\ldots,b_{m})$, $\^G^s_{k\times q}$ are the inequality constraints. }\label{eq:2}
\end{align}
Pick $(m-k)$ columns of $\^R^s$ so that resulting matrix is non singular. Then we partition $\^R^s$ and $\^G^{s}$ as $\^R^s=[\^R^0_{11}\hspace{2 mm} \^R^0_{12}]$, $\^G^s=[\^R^0_{21}\hspace{2 mm} \^R^0_{22}]$, where $\^R^0_{11}$ is a $(m-k)\times(m-k)$ dimensional non singular matrix. Now correspondingly, partition $\bm\beta_1$ as $\bm\beta_1^T=(\bm\beta_3^T \hspace{2 mm}\bm\gamma_2^T)$. Then \ref{eq:1} and \ref{eq:2} can be reformulated as
\begin{align}
   \^R^0_{11}\bm\beta_3+ \^R^0_{12}\bm\gamma_2&=\*b_s\\
   \^R^0_{21}\bm\beta_3+ \^R^0_{22}\bm\gamma_2&>\*g_s.
\end{align}
Eliminating $\bm\beta_3$ \{$\bm\beta_3={\^R^0_{11}}^{-1}(\*b_s-\^R^0_{12}\bm\gamma_2)$\}, the non binding constraints can be written as $\^D_0\bm\gamma_2 \geq \*w$, where $\^D_0=\^R^0_{22}-\^R^0_{21}{\^R^0_{11}}^{-1}\^R^0_{12}$, $\*w=\*g_s-\^R^0_{21}{\^R^0_{11}}^{-1}\*b_s$. Define $\bm\gamma^T=(\bm\beta_2^T \hspace{2 mm} \bm\gamma_2^T)$, then the inequality constraint on $\gamma$ is given by $\^D\bm\gamma \geq \*w$, where $\^D=[0 \hspace{3 mm}\^D_0]$. Let $\^X$ be partitioned corresponding to this reparametrization as $\^X=[\^X_{11} \hspace{3 mm}\^X_{12} \hspace{3 mm}\^X_2]$, where $\^X_{11}$ has $(m-k)$ columns corresponding to $\bm\beta_3$. Then we can write the linear predictor as,
\begin{align*}
    \^X\bm\beta&=\^X_2\bm\beta_2+ \^X_{11}\bm\beta_3 +\^X_{12}\bm\gamma_2\notag\\
    &=\^X_2\bm\beta_2+ \^X_{11}{\^R^0_{11}}^{-1}(\*b_s-\^R^0_{12}\bm\gamma_2) +\^X_{12}\bm\gamma_2\notag\\
    &=\^U\bm\gamma+ \bm\delta,
\end{align*}
where $\^U=[\^X_2\hspace{4mm}\^X_{12}-\^X_{11}{\^R^0_{11}}^{-1}\^R^0_{12}]$, $\bm\delta=\^X_{11}{\^R^0_{11}}^{-1}\*b_s$. Note that the original parameter $\bm\beta$ can be expressed in terms of $\bm\gamma$ as $\bm\beta=\*A\bm\gamma+ \nu$, where $\nu=({\^R^0_{11}}^{-1}\*b_s,\*0,\*0)^T$, and the matrix $\*A$ is given by $\*A=\begin{bmatrix}
0 & -{\^R^0_{11}}^{-1}\^R^0_{12} \\
0 & I \\
I & 0
\end{bmatrix}$.

Using the above representation of $\^X\bm\beta$, linear model or the likelihood for GLM can be reparametrized in terms of $\bm\gamma$
%\begin{equation}
%L(\bm\gamma) \propto e^{\{\*Y^T[\^U\bm\gamma+ %\bm\delta]-\sum_{i=1}^{n}\Psi(\*u_i^T\bm \gamma+\*\delta_i)\} }.  
%\end{equation}
and inference can be made on $\bm\gamma$ under the linear inequality constraints $\^D\bm\gamma \geq \*w$, using the BICLS or BICGLM method proposed in the article and treating $\*\delta_i$ as offsets. 

\section{Additional Tables}
\begin{table}[H]
\centering
\begin{tabular}{|c|c|c|c|c|}
\hline
Sample size         & Parameter &  \begin{tabular}[c]{@{}c@{}}BICLS\end{tabular} & \begin{tabular}[c]{@{}c@{}}ICLS\end{tabular} & \begin{tabular}[c]{@{}c@{}}OLS\end{tabular} \\ \hline
\multirow{3}{*}{10}  & $\beta_1$  & 0.91   &  0.89  & 1.12                                                 \\ \cline{2-5} 
& $\beta_2$ & 0.89    &0.85                                          &1.01                                              \\ \cline{2-5} 
                    & $\beta_3$                                          &1.12                                                  & 1.04                                                 & 1.07                                                \\ \hline
\multirow{3}{*}{30} & $\beta_1$                 & 0.50                                                     &  0.53                                                  & 0.56                                                   \\ \cline{2-5} 
                    & $\beta_2$                       & 0.52                                & 0.56                             & 0.64                             \\ \cline{2-5} 
                    & $\beta_3$                      &0.67                                & 0.67                               & 0.69                               \\ \hline
\multirow{3}{*}{50} & $\beta_1$                 & 0.43                                                     & 0.45                                                    & 0.45                                                   \\ \cline{2-5} 
                    & $\beta_2$                       & 0.39                               & 0.43                               & 0.46                             \\ \cline{2-5} 
                    & $\beta_3$                      & 0.47                                 & 0.48                               & 0.48                              \\ \hline
\end{tabular}
\caption{Comparison of average standard error of the estimates, Scenario A1.}
\label{tab:my-tablea1}
\end{table}

\begin{table}[H]
\begin{center}
\begin{tabular}{|c|c|c|c|c|c|}
\hline
a,b         & $\beta$  & \begin{tabular}[c]{@{}c@{}}ICLS\\ (MSE)\end{tabular} & \begin{tabular}[c]{@{}c@{}}OLS\\ (MSE)\end{tabular}  & \begin{tabular}[c]{@{}c@{}}ICLS\\ (Variance)\end{tabular} & \begin{tabular}[c]{@{}c@{}}OLS\\ (Variance)\end{tabular} \\ \hline
\multirow{3}{*}{0.02}             & $\beta_1$                                                  & 1.2                                                & 1.2                                                                                                     & 1.3                                                     & 1.3                                                    \\ \cline{2-6} 
                    & $\beta_2$                             & 1.3                            & 1.5                                                           & 1.5                                & 1.8                              \\ \cline{2-6} 
                    & $\beta_3$                             & 1                            & 1.1                                                          & 1.1                                & 1.1                                       \\ \hline
\multirow{3}{*}{0.005}            & $\beta_1$                                                  & 1.2                                                & 1.2                                                                                                     & 1.3                                                     & 1.3                                                    \\ \cline{2-6} 
                    & $\beta_2$                             & 1.3                            & 1.5                                                           & 1.5                                & 1.8                              \\ \cline{2-6} 
                    & $\beta_3$                             & 1                            & 1.1                                                          & 1.1                                & 1.1                              \\ \hline
\multirow{3}{*}{0.0025} & $\beta_1$                                                  & 1.2                                                & 1.2                                                                                                     & 1.3                                                     & 1.3                                                    \\ \cline{2-6} 
                    & $\beta_2$                             & 1.3                            & 1.5                                                           & 1.5                                & 1.8                              \\ \cline{2-6} 
                    & $\beta_3$                             & 1                            & 1.1                                                          & 1.1                                & 1.1                               \\ \hline                    
\end{tabular}
\end{center}
\caption{Prior sensitivity analysis exploring relative efficiency ratios of estimates (compared to BICLS) for Scenario A1 (n=50) for various choices of the hyperparameters a, b in the prior specification (4). The results remain unchanged illustrating relative insensitivity of the priors on posterior inference.}
\label{tab:my-tableS1}
\end{table}



\begin{table}[H]
%\small
\centering
\begin{tabular}{|c|c|c|c|c|}
\hline
Sample Size         & \begin{tabular}[c]{@{}c@{}}Parameter\end{tabular}  & \begin{tabular}[c]{@{}c@{}}BICLS \end{tabular} & \begin{tabular}[c]{@{}c@{}}ICLS\end{tabular} & \begin{tabular}[c]{@{}c@{}}OLS\end{tabular} \\ \hline
\multirow{4}{*}{50} & $\beta_0$                                                                                             & 0.437                                                    & 0.429                                                  & 0.429                                                  \\ \cline{2-5} 
                    & $\beta_1$                                                                                      & 0.314                                                 & 0.312                                                 & 0.453                                                \\ \cline{2-5} 
                    & $\beta_2$                                                                                         &0.254                                                  &0.252                                                &0.459                                               \\ \cline{2-5} 
                    & $\beta_3$                                                                                        & 0.313                                                  & 0.316                                                  &0.485                                                \\ \hline
\end{tabular}
\caption{Comparison of average standard error of the estimates, Scenario B.}
\label{tab:my-tableA2}
\end{table}
\begin{table}[H]
\centering
\begin{tabular}{|l|l|l|l|}
\hline
Parameter    & BICGLM & ICGLM & GLM   \\ \hline
$\beta_1$    & 0.033  & 0.051 & 0.073 \\ \hline
$\beta_2$    & 0.068  & 0.106 & 0.188 \\ \hline
$\beta_3$    & 0.080  & 0.120 & 0.203 \\ \hline
$\beta_4$    & 0.070  & 0.107 & 0.166 \\ \hline
$\beta_5$    & 0.072  & 0.107 & 0.188 \\ \hline
$\beta_6$    & 0.065  & 0.111 & 0.181 \\ \hline
$\beta_7$    & 0.068  & 0.095 & 0.204 \\ \hline
$\beta_8$    & 0.056  & 0.087 & 0.188 \\ \hline
$\beta_9$    & 0.075  & 0.116 & 0.166 \\ \hline
$\beta_{10}$ & 0.066  & 0.104 & 0.175 \\ \hline
$\beta_{11}$ & 0.106  & 0.160 & 0.201 \\ \hline
\end{tabular}
\caption{Comparison of average standard error of the estimates, Scenario C, n=100.}
\label{tab:my-tableA3}
\end{table}

\section{Additional Figures}
\begin{figure}[H]
\centering
\includegraphics[width=.9\linewidth , height=.9\linewidth]{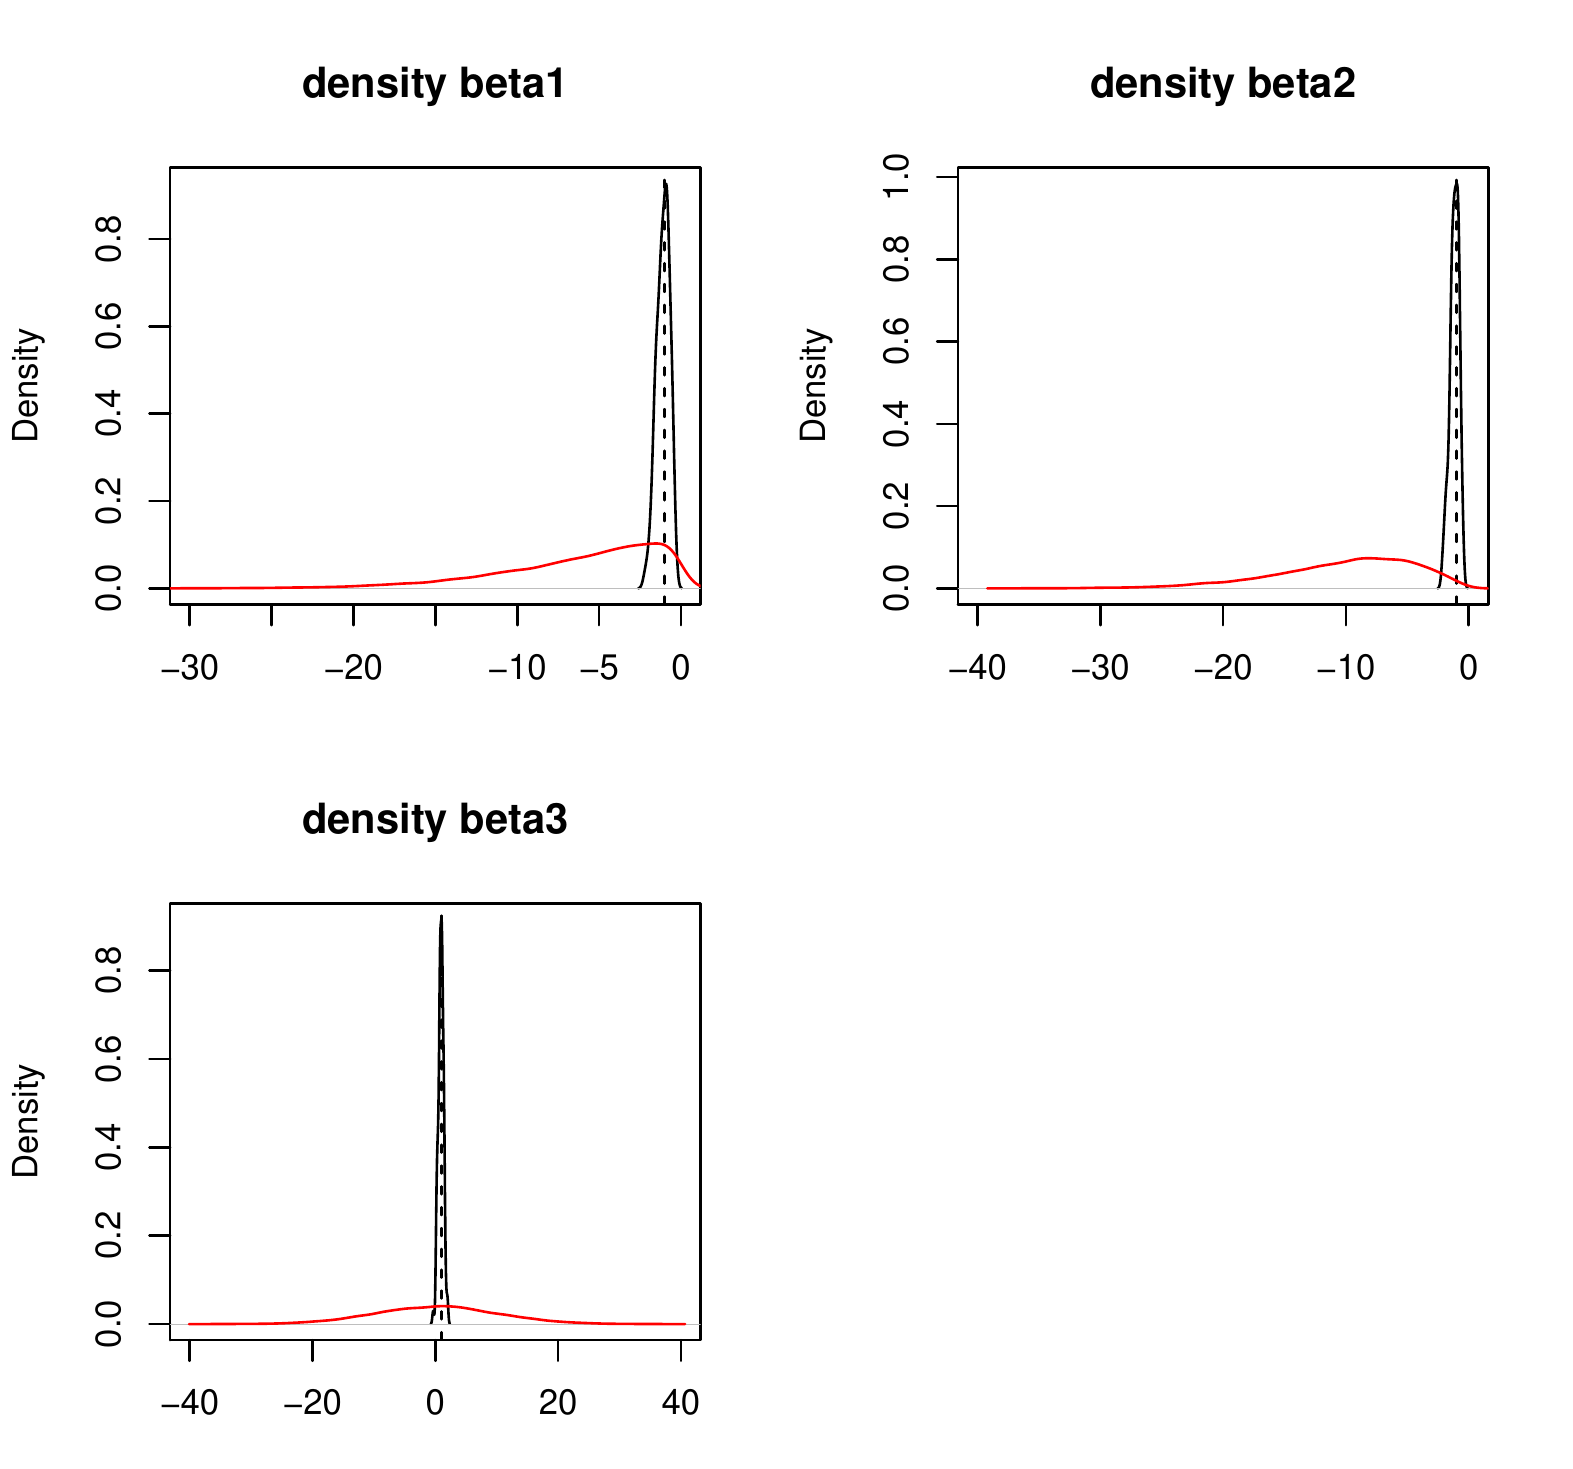}
\caption{Density plots exploring prior sensitivity, Scenario A1  
(n=50). The marginal prior densities are shown in red and the marginal posterior densities are shown in black along with the true value of the parameter $\bm\beta$ = (-1,-1,1), which is overlaid. The posterior is highly concentrated around the true value irrespective of the vague prior.}
\label{fig:fig1}
\end{figure}


\begin{figure}[H]
\centering
\includegraphics[width=.9\linewidth , height=.9\linewidth]{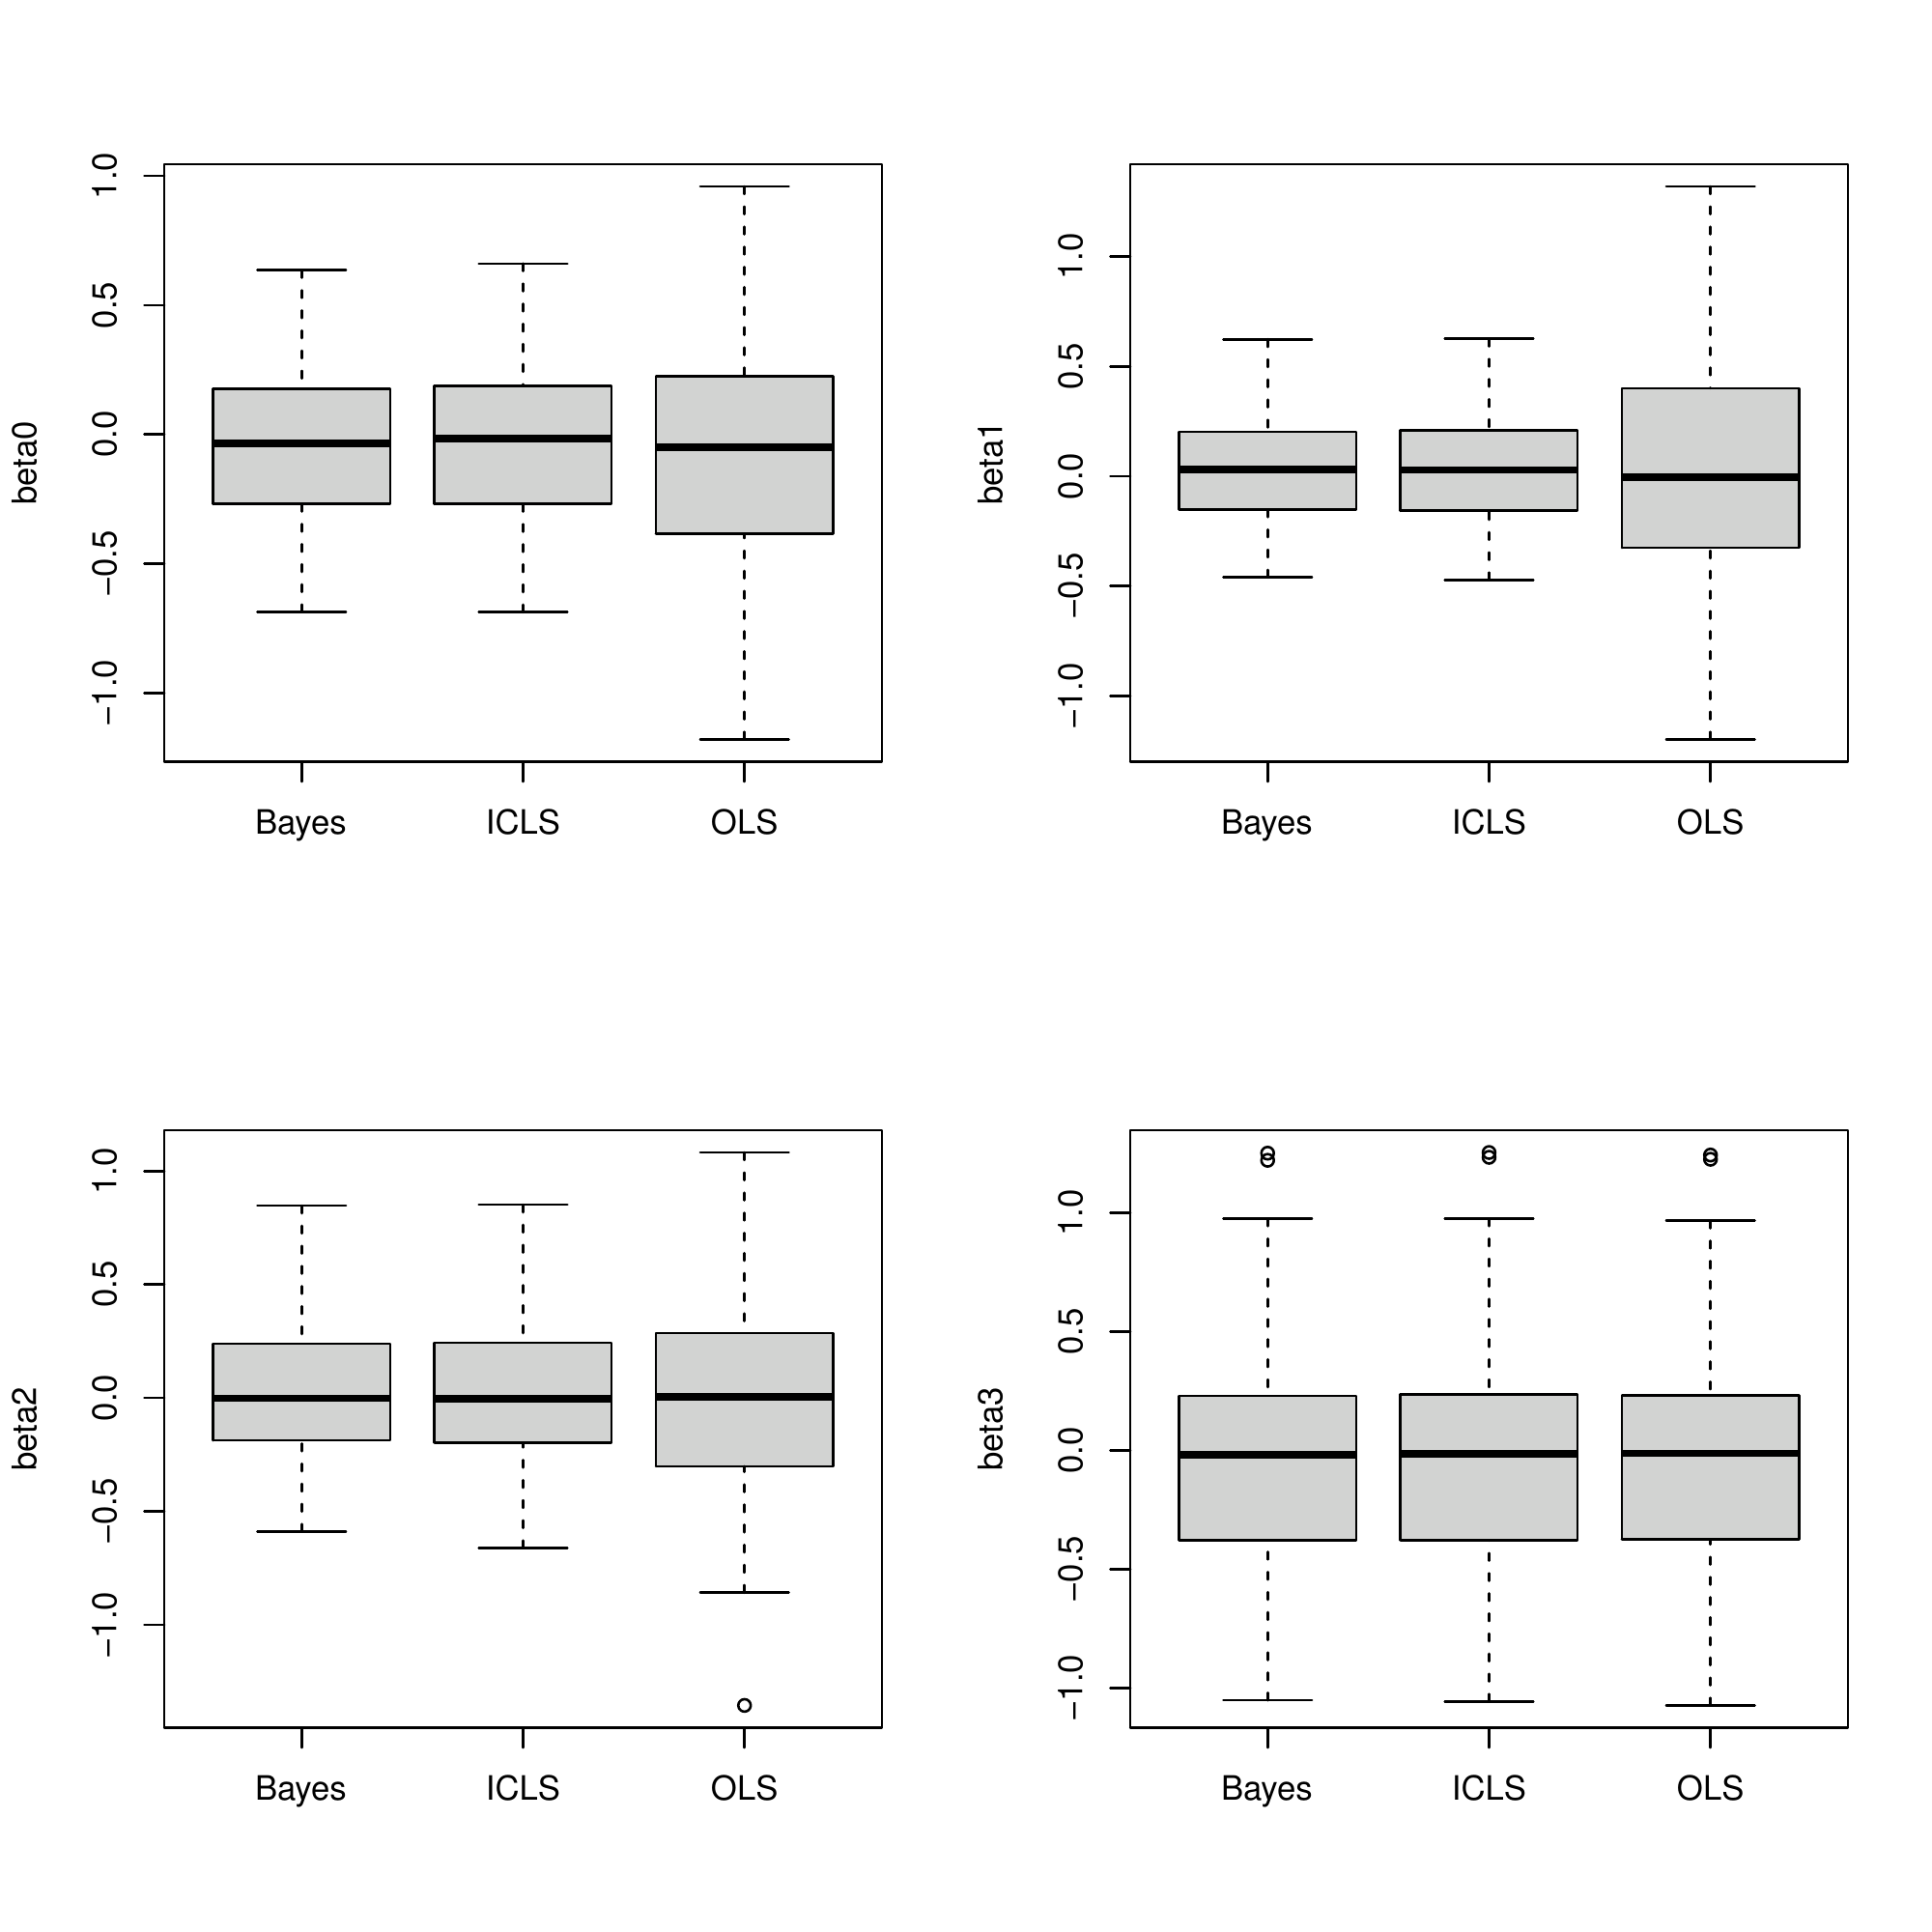}
\caption{Boxplot of biases of the estimated parameters, Scenario B. 
}

\label{fig:fig2}
\end{figure}

\begin{figure}[H]
\centering
\includegraphics[width=.9\linewidth , height=.9\linewidth]{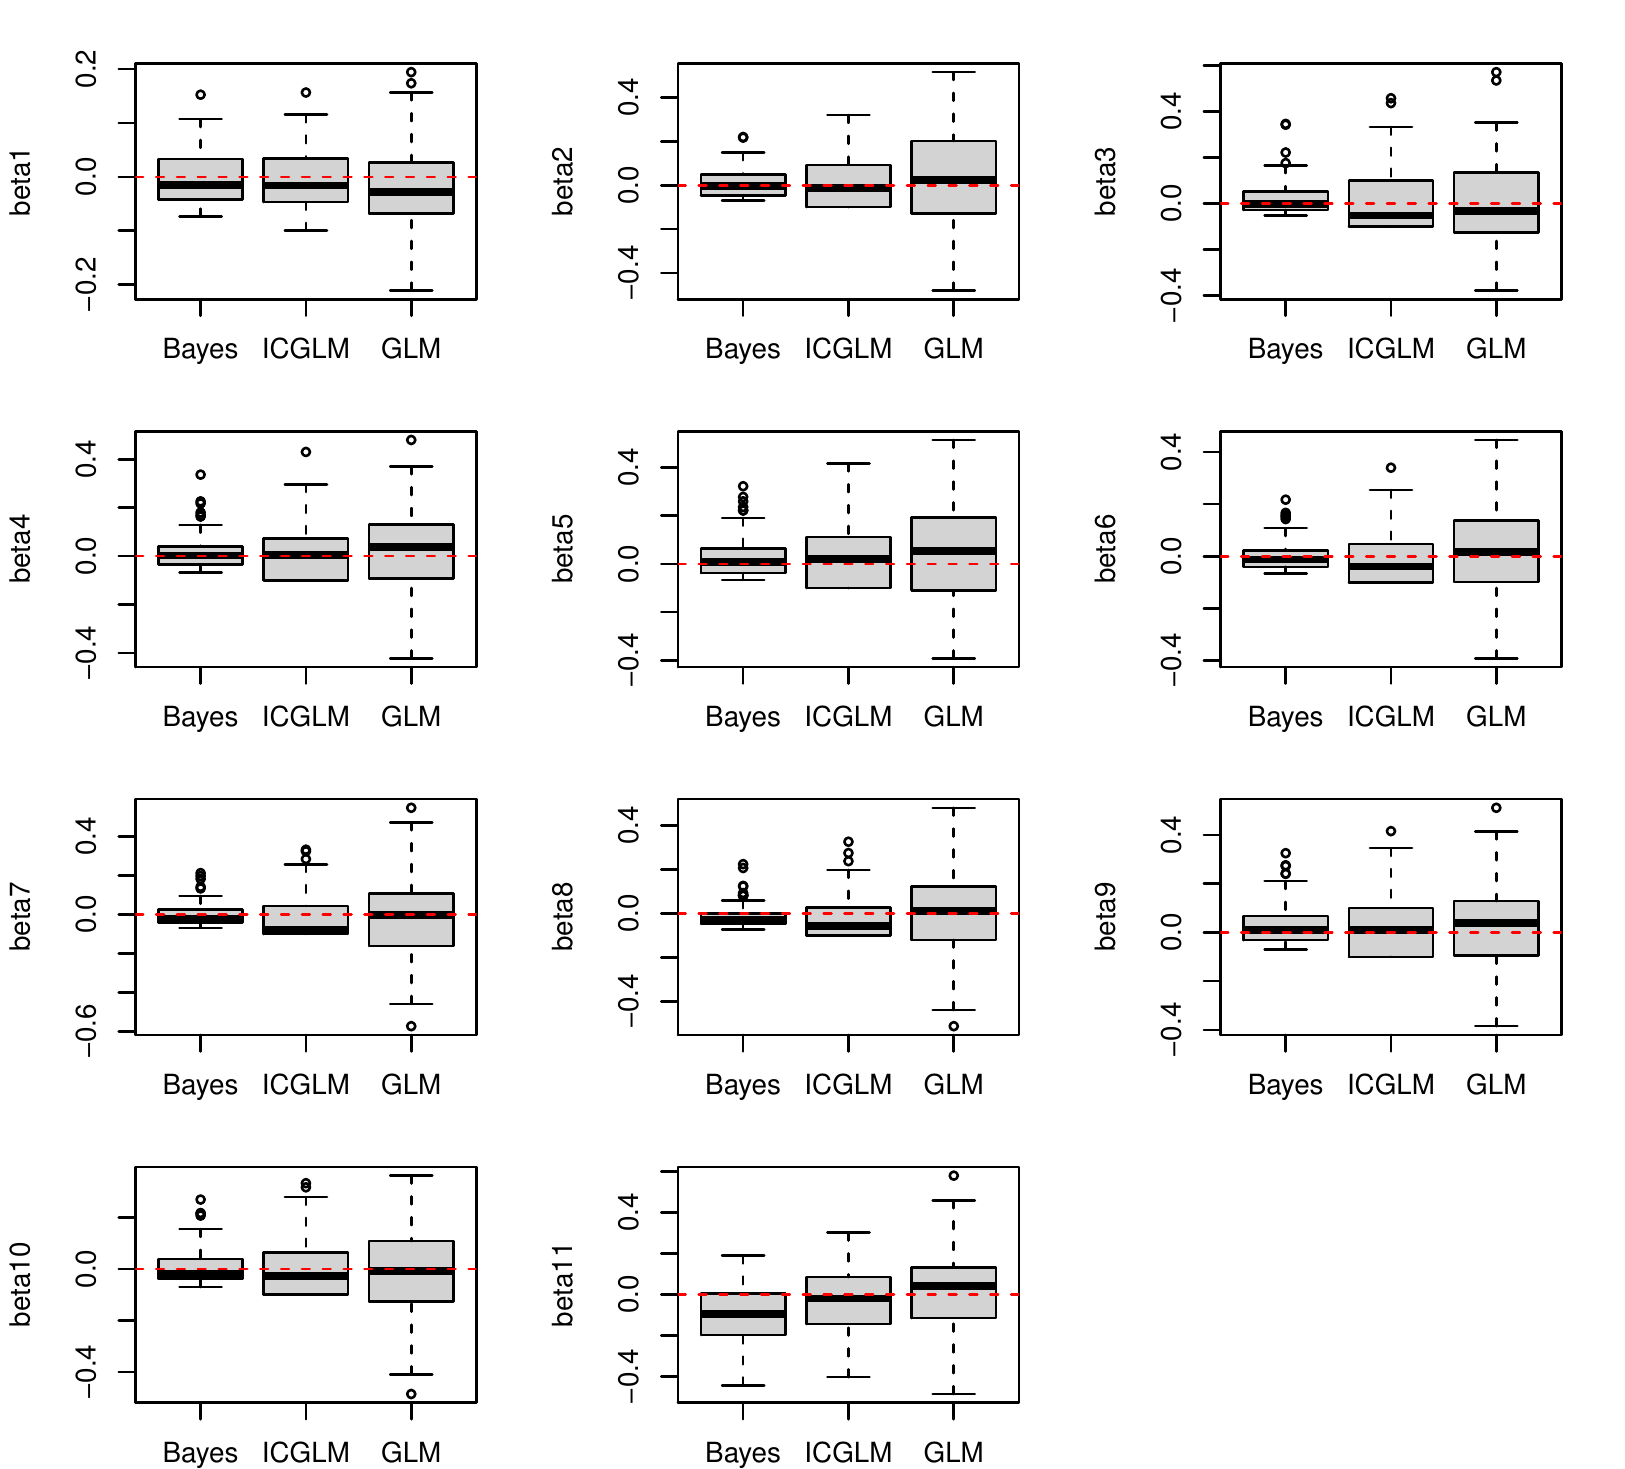}
\caption{Boxplot of biases of the estimated parameters, Scenario C. }
\label{fig:fig3}
\end{figure}


\begin{figure}[H]
\centering
\begin{tabular}{lll}
\includegraphics[width=.4\linewidth , height=.4\linewidth]{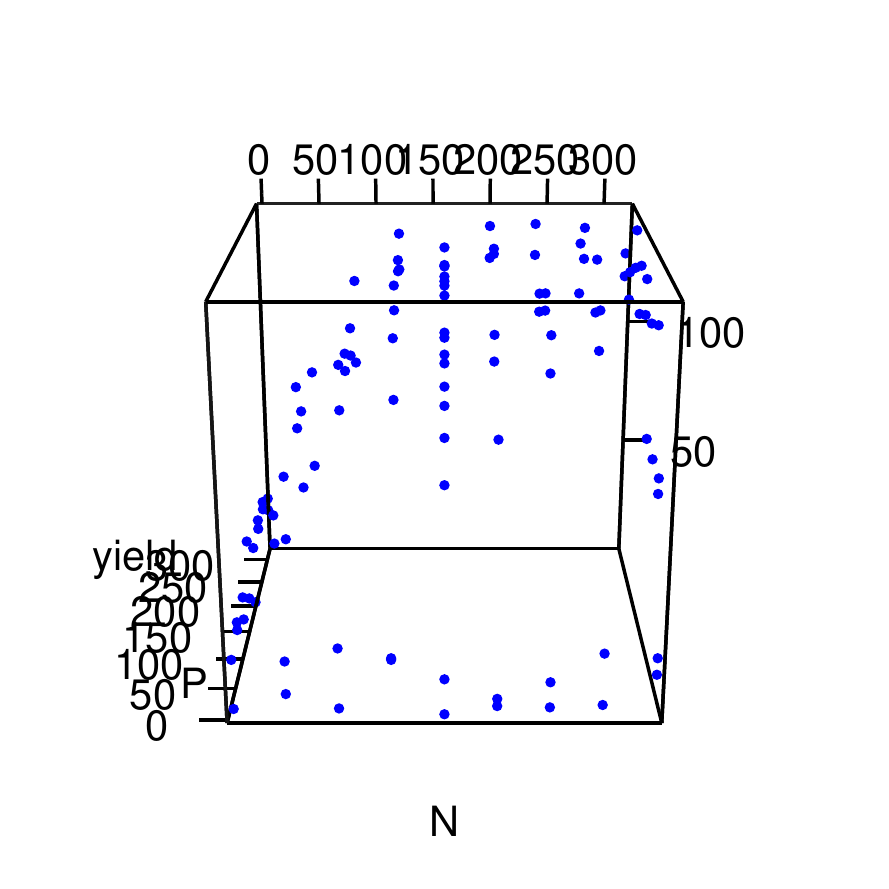}&
\includegraphics[width=.3\linewidth , height=.4\linewidth]{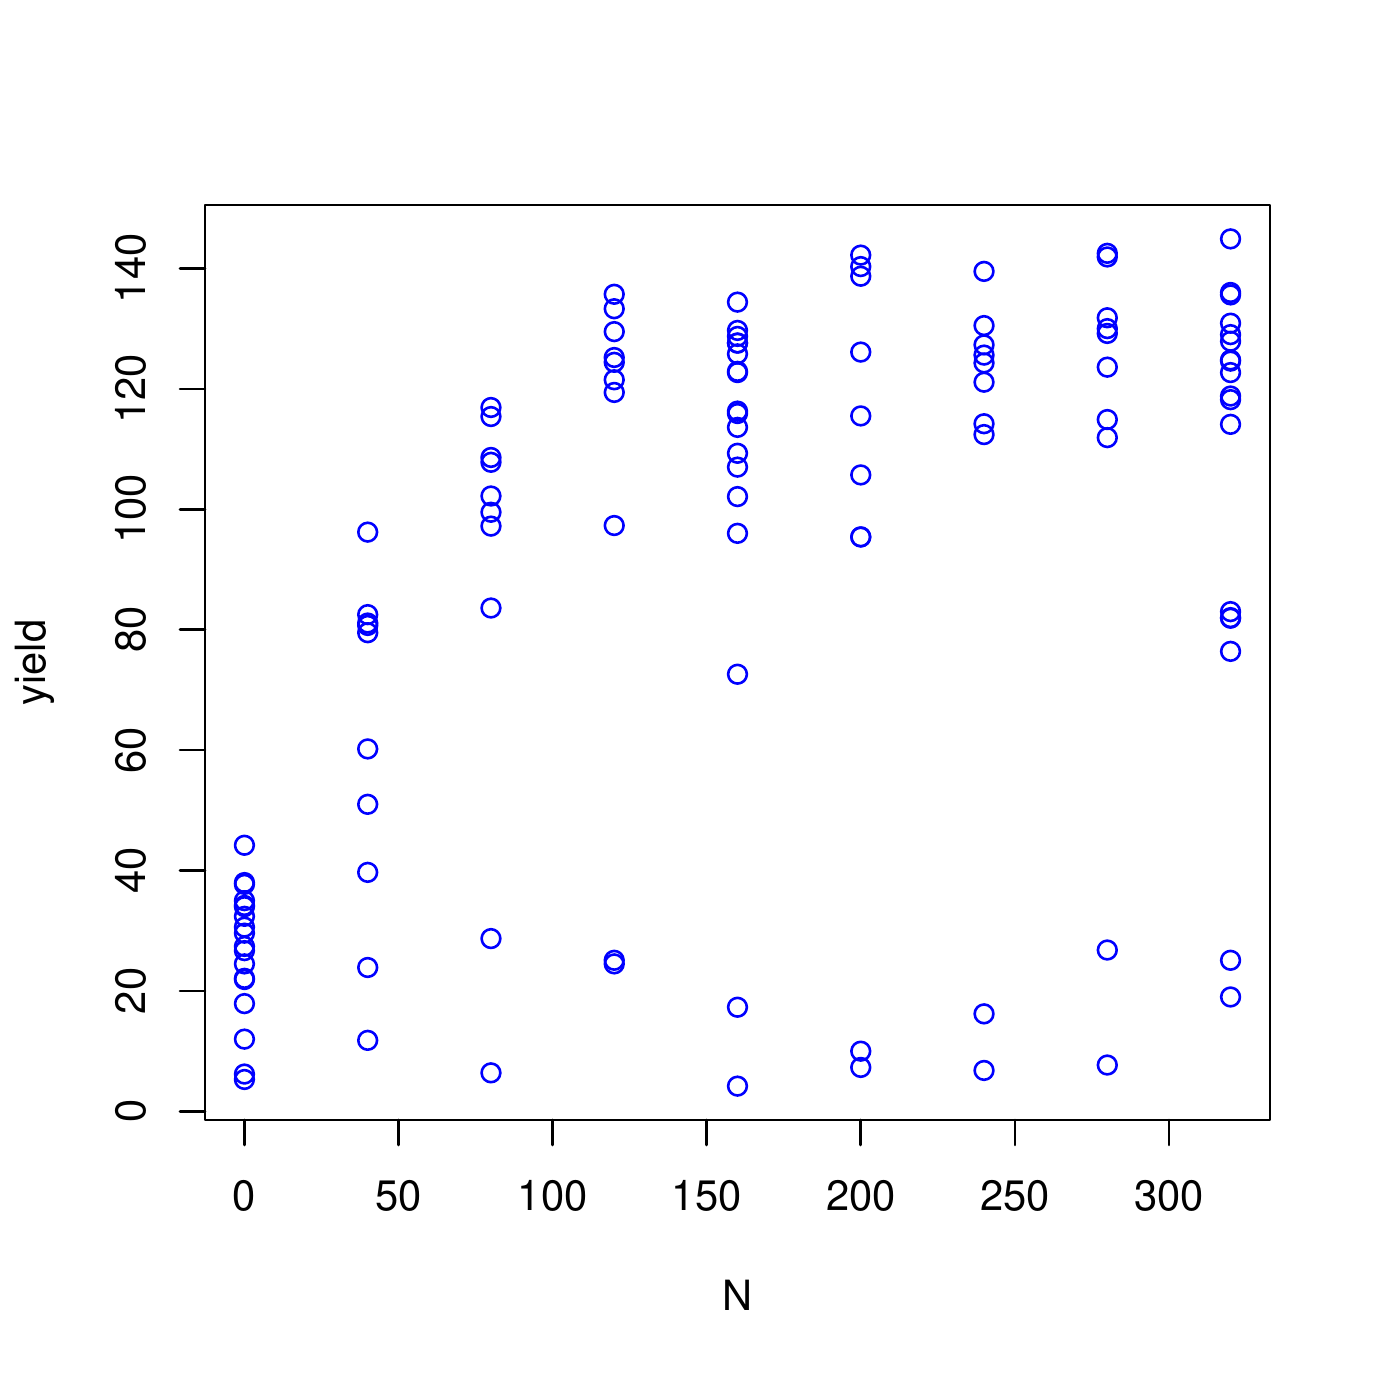}&
\includegraphics[width=.3\linewidth , height=.4\linewidth]{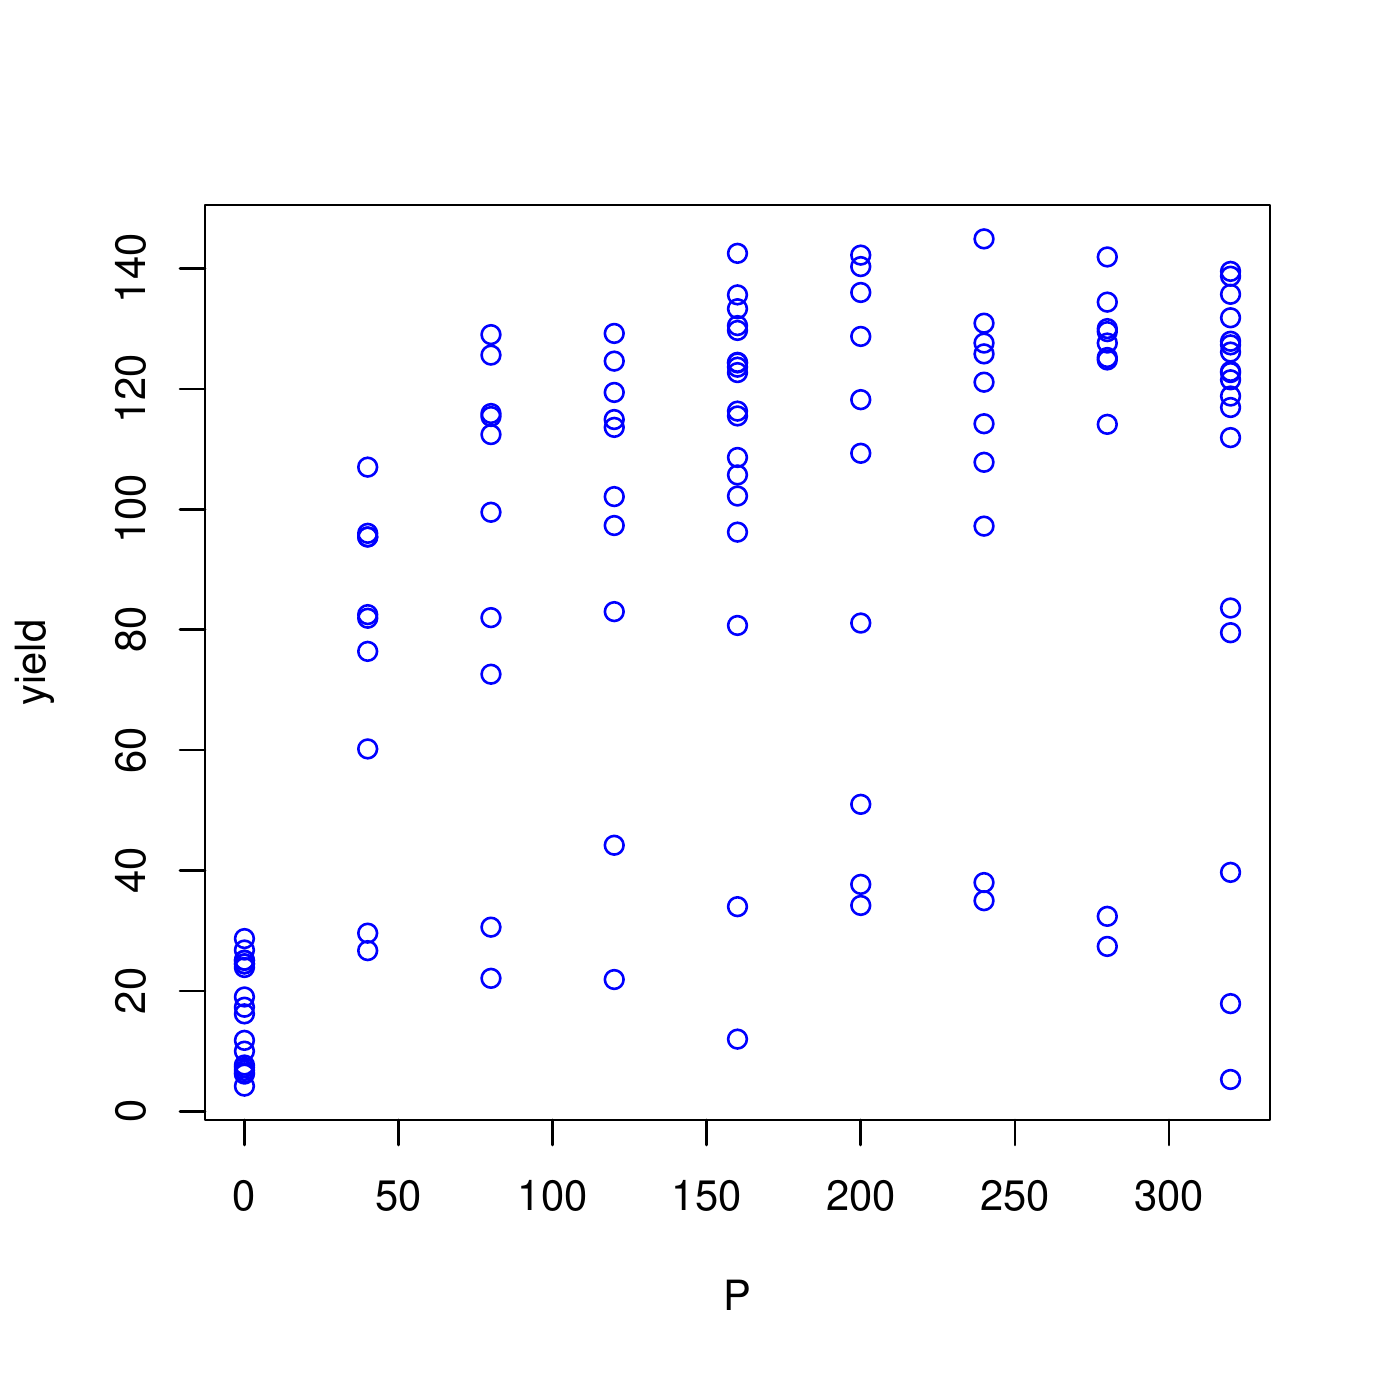}\\
\end{tabular}
\caption{Corn yield as function of N and P fertilizer amounts.}
\label{fig:fig4}
\end{figure}

\begin{figure}[ht]
\centering
\includegraphics[width=.9\linewidth , height=.6\linewidth]{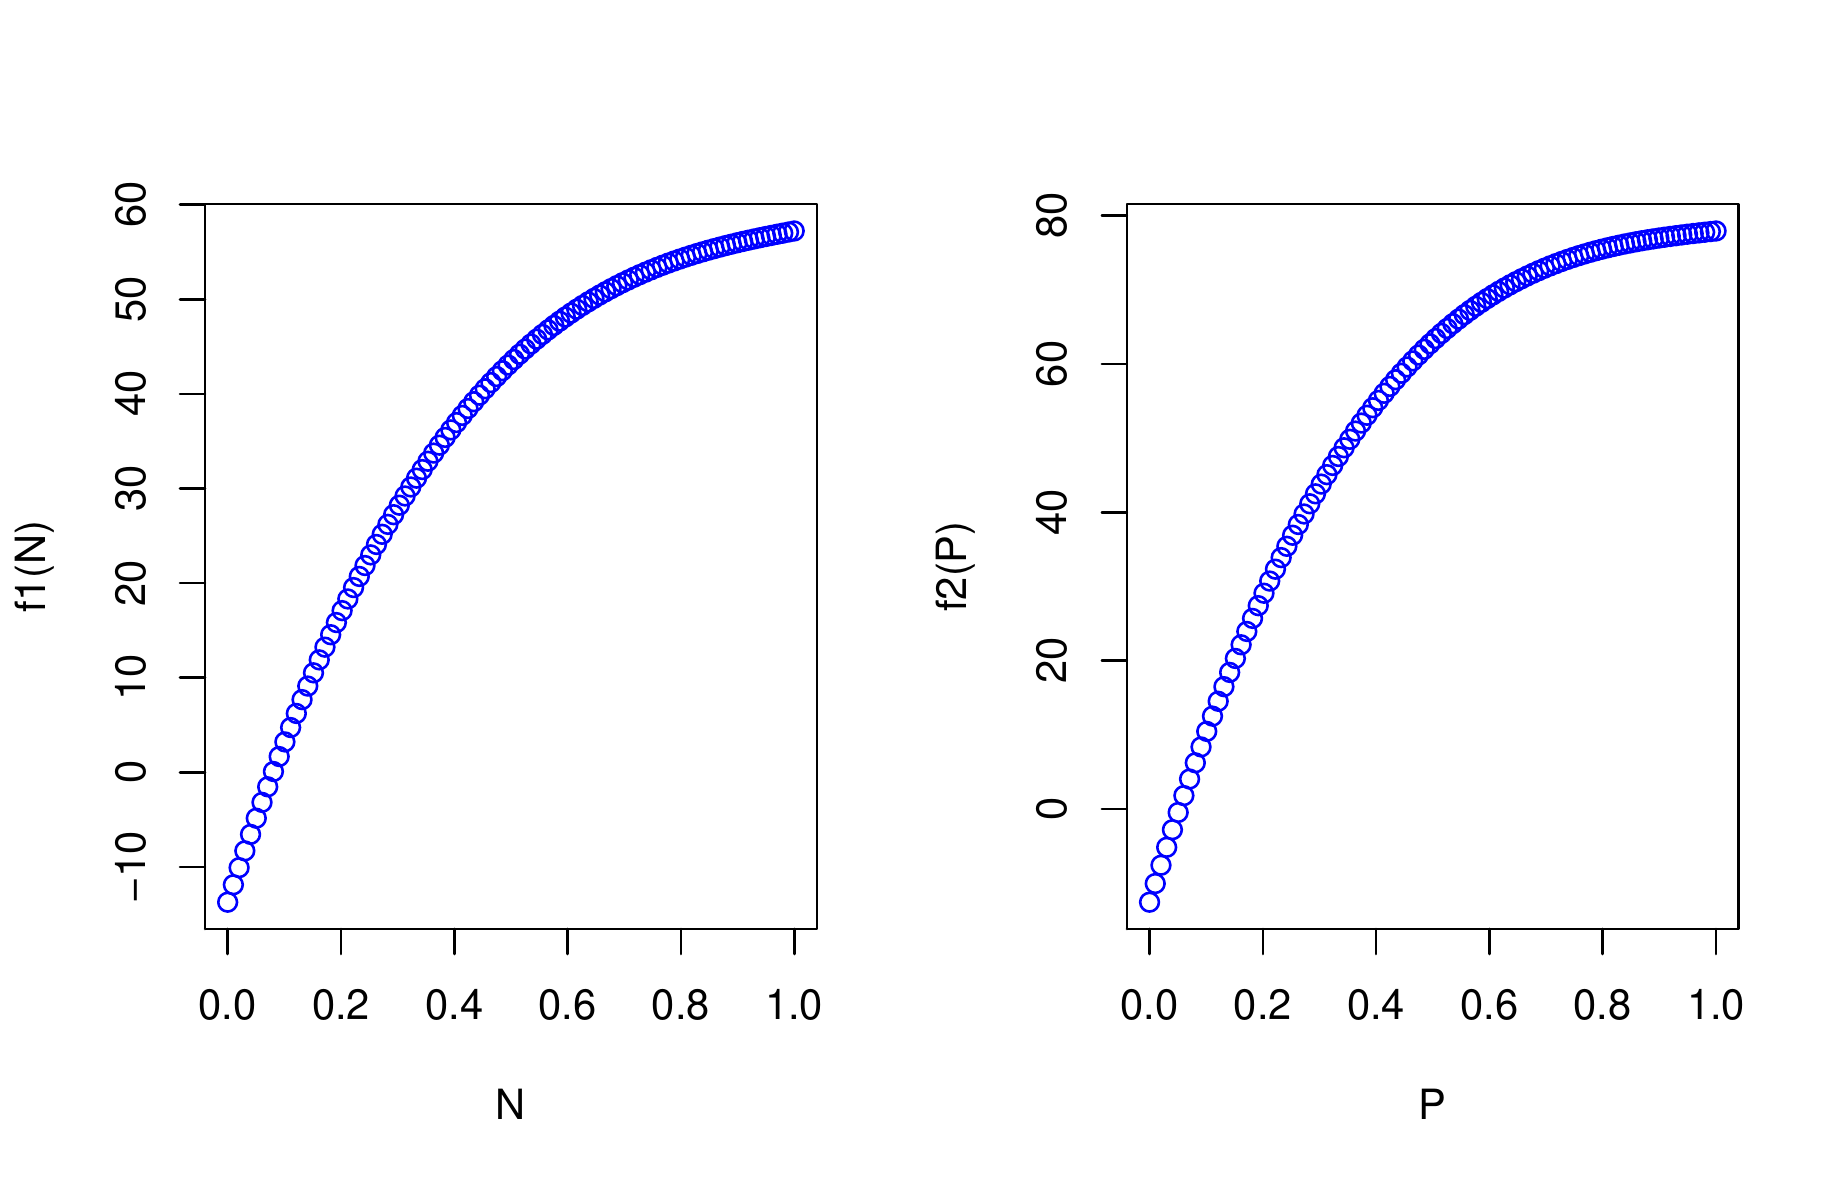}
\caption{Estimated additive effects of N and P for the heady data.}
\label{fig:fig7new}
\end{figure}


\begin{figure}[H]
\centering
\includegraphics[width=.5\linewidth , height=.5\linewidth]{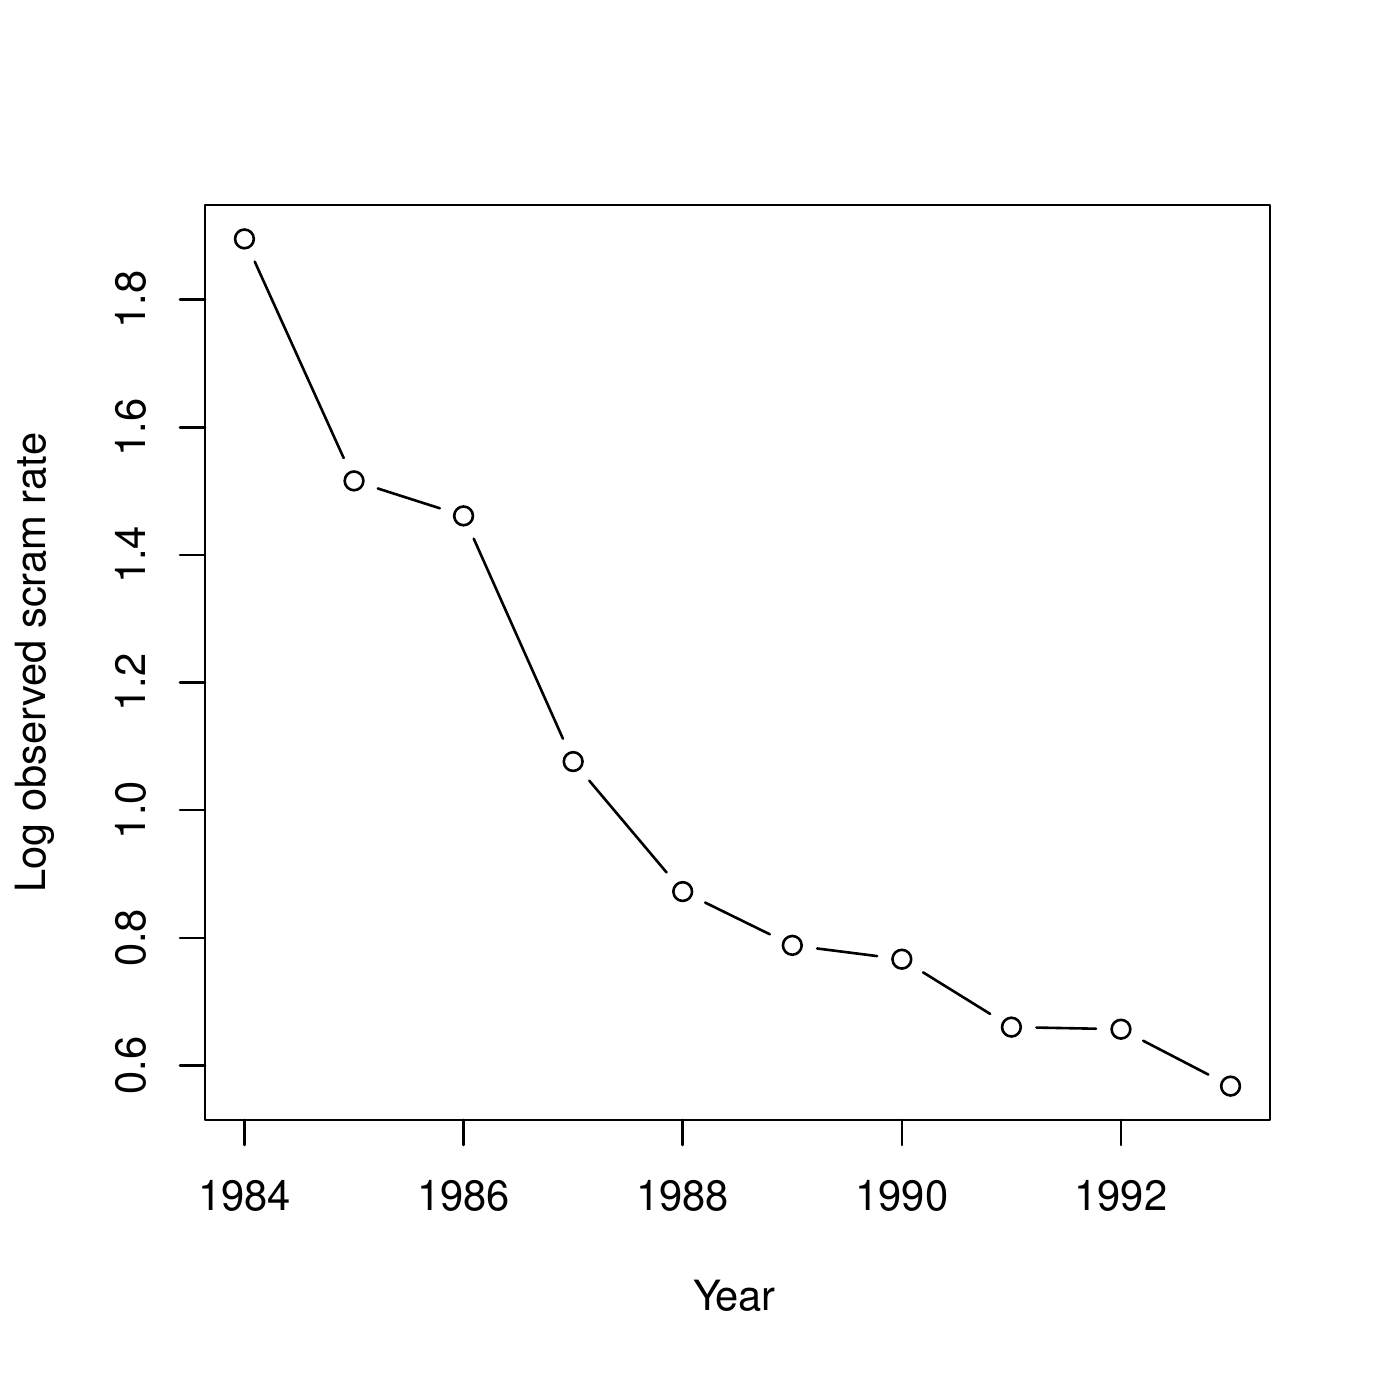}
\caption{Plot of observed log scram rate averaged over plants for different years.}
\label{fig:fig9}
\end{figure}


\newpage
\bibliographystyle{JASA}
\bibliography{lit}% place <bib-data-file> 

% ** Acknowledgements **
% \begin{acknowledgement}
% \end{acknowledgement}


\end{document}
